# Supplementary material for: Matrix Norms in Data Streams: Faster, Multi-Pass and Row-Order
Source: arXiv:1609.05885 source file (2018-10-24)
Supplement: Supplementary file 1 [file appendix_general_norm.tex]

\section{Proofs from Section~\ref{sec: unitarily invariant} (Unitarily Invariant Norms)}
\label{sec:proofs of sec ui}

\subsection{Proof of Theorem~\ref{thm:norm psd}}
The next lemma is an immediate consequence 
of~\cite[Lemma 6.2]{woodruff2014sketching}.
\begin{lemma}
\label{lemma:ose singular values}
Let $S\in\R^{t\times d}$ be an $(\epsilon, \delta, d)$-OSE matrix. 
%then $t\ge d$. 
Let $\sigma_i$ denote the $i$-th largest singular value of $S$.
Then with probability at least $1-\delta$,  
\[
  \forall i\in [d],\qquad 
  \sigma_i \in[1-\epsilon, 1+\epsilon] .
\]
\end{lemma}

\begin{oseeigenvalueslemma}
%\label{lemma:ose preserves eigenvalues}
\osepreserveseigenvalueslemma
\end{oseeigenvalueslemma}
\begin{proof}
By the Spectral Theorem, we can write $A=P\Lambda P^T$, where $P\in\R^{n\times r}$ is a matrix with orthonormal columns and $\Lambda\in\R^{r\times r}$ is a diagonal matrix.
The matrix $SP\in\R^{t\times r}$ is an $(\epsilon,\delta, r)$-OSE by Lemma~\ref{lemma:ortho trans ose}.
Lemma \ref{lemma:ose singular values} implies that, with probability at least $1-\delta$,  $\sigma_i(SP)\in(1\pm \epsilon)$ for all $i\in[r]$.
The lemma follows by applying Lemma 3.2 of \cite{andoni2013eigenvalues}.

\end{proof}

\begin{upperboundallnormlemma}
\upperboundallnormslemmatext
\end{upperboundallnormlemma}
%\lynote{I changed the OSE from $d$ to $d'$.}

\begin{proof}
We can write $A=U\Lambda U^T$ 
where $U$ is an orthogonal matrix and $\Lambda$ is a diagonal matrix. 
By Lemma~\ref{lemma:ortho trans ose}, 
also $SU$ is an $(\epsilon, d\delta/n, d')$-OSE matrix,
and thus it suffices to consider diagonal matrices, i.e., $A=\Lambda$
(the general case follows by replacing $S$ throughout the proof with $SU$).
For simplicity, we assume $n$ is a multiple of $d$ 
(the general case only requires to round $n/d$ upwards), 
and write $\Lambda = \sum_{k=1}^{n/d} \Lambda^{(k)}$,
where each matrix $\Lambda^{(k)}$ is obtained from $\Lambda$ 
by breaking it into blocks of size $d\times d$ 
and zeroing all but the $k$-th main-diagonal block.
Then by the triangle inequality,
\[
  l(S\Lambda S^T)
  = l\Big( \sum_{k=1}^{n/d} S\Lambda ^{(k)} S^T \Big)
  \leq \sum_{k=1}^{n/d} l\left( S \Lambda^{(k)} S^T \right).
\]
For each $k$, by Lemma~\ref{lemma:ose preserves eigenvalues}, 
with probability at least $1-d\delta/n$,
the entire non-zero spectrum of $S\Lambda^{(k)} S^T$ approximates 
that of $\Lambda^{(k)}$ within factor $(1\pm 3\eps)$.
Now assuming this event occurs, 
we use (twice) the monotonicity of the norm $l(\cdot)$ in the singular values, 
and obtain
\[
  l(S \Lambda ^{(k)} S^T)
  \leq (1+3\eps))\ l(\Lambda^{(k)}) 
  \leq (1+3\eps) \norm{\Lambda}_{2} l(I_d) .
\]
%By a union bound, with probability at least $1-\delta$,
%these events occur for all $k\in[n/d]$, and 
The lemma follows by a union bound over these $n/d$ events.
\end{proof}

\begin{variationalnormprop}
\variationalcharpropositiontext
\end{variationalnormprop}

\begin{proof}
  Let $\varphi$ denote the maximum value attained in the expression on the right side above.
  Note that $\varphi$ is well defined since the feasible region is compact.
  Let $A = U D V^T$ denote the s.v.d.\ of $A$ with $U_1,\ldots,U_m\in\calS^{m-1}$ and $V_1,\ldots,V_n\in\calS^{n-1}$ the columns of $U$ and $V$, respectively, and $D$ a $m\times n$ diagonal matrix containing the singular values of $A$.
  Choosing $u_i=U_i$ and $v_i=V_i$, for all $i=1,2,\ldots,m$, we see $\|A\| = \|\sigma\|\leq\varphi$, where $\sigma$ denotes the $m$-dimensional vector of singular values of $A$.

  For the reverse direction, let $(u_i)_{i\in [m]}$, $(v_i)_{i\in[m]}$ be some optimal solution.
  We decompose the vectors in the optimal solution as $u_i = \sum_{j=1}^m \alpha_{ij}U_j$ and $v_i = \sum_{j=1}^n\beta_{ij}V_j$, where $\sum_j\alpha_{ij}^2 = 1 = \sum_j\beta_{ij}^2$ for all $i$.
  Thus, $u_i^T A v_i = \sum_{j=1}^m \alpha_{ij}\beta_{ij}\sigma_j$.
  Furthermore, $\sum_j |\alpha_{ij}\beta_{ij}| \leq 1$ and $\sum_i|\alpha_{ij}\beta_{ij}|\leq 1$ by the Cauchy-Schwarz Inequality.

  Let $\Lambda$ be the $m\times m$ matrix with $ij$th entry $|\alpha_{ij}\beta_{ij}|$.
  The above inequalities imply that $\Lambda$ is doubly substochastic, and by definition
  \[(\Lambda\sigma)_i =\sum_{j}|\alpha_{ij}\beta_{ij}|\sigma_j \geq\sum_{j}\alpha_{ij}\beta_{ij}\sigma_j = u_i^TAv_i.\]
  It is well known (Horn \& Johnson, ``Topics in Matrix Analysis'' p.165) that $\Lambda$ can be decomposed as a convex combination of partial permutation matrices, i.e.\ matrices form by zeroing out some entries of a permutation matrix.
  Thus, we may write a convex combination of permutation matrices $\Lambda' = \sum \lambda_kP_k \geq \Lambda$, where $P_k$ are permutation matrices (augment the partial permutation matrices to permutation matrices arbitrarily) and the inequality holds coordinate-wise implying also that $\Lambda'\sigma \geq \Lambda\sigma$ coordinate-wise.

  Now, by monotonicity of symmetric norms, the traingle inequality, and permutation symmetry we have 
\[\varphi = \|(|u_1^T A v_1|, |u_2^T A v_2|, \ldots, |u_m^TAv_m|)^T\| \leq \sum_k \lambda_k\|P_k\sigma\| = \|\sigma\| = \|A\|,\]
  which is the desired inequality.
\end{proof}

\subsection{General Matrices and $Q$-norms}\label{app:qnorm}

In this section we will show an even smaller sketch suffices when $\ell$ is a $Q$-norm.
\begin{theorem}
\label{thm:norm non-psd Q-norm}
Let $A\in \bbR^{n\times n}$ be a PSD matrix. 
Let $\tilde{\ell}:\bbR^{n\times n}\rightarrow \bbR_{\ge 0}$ be a unitarily invariant norm and $\ell:\bbR^{n\times m}\rightarrow \bbR_{\ge0}$ be a $Q$-norm defined as  $\ell(A):=\sqrt{\tilde{\ell}(AA^T)}$. 
Let $G\in \bbR^{t\times n}$ and $H\in\bbR^{t\times m}$ be two independent $(\epsilon, \delta, O(d\log n))$-OSEs.
%For any $t=\Omega(\log n/\epsilon^2)$ satisfing $\varepsilon^{(2)}_\ell(t)\ge r_2(l, A)/\epsilon^3$ and $t'= \Omega(t+\log n)/\epsilon^2$, 
With probability at least $1-2n\delta$, 
\[
(1-O(\epsilon))\ell(A)^2\le \tilde{\ell}(GAH^THA^TG^T)\le (1+O(\epsilon))\ell(A)^2 + O\left(\frac{\ell(I_d)^2}{d}\sum_{i=d+1}^n\sigma_i(A)^2\right). 
\]
\end{theorem}

\begin{proof}[Proof of Theorem~\ref{thm:norm non-psd Q-norm}]
We will apply the inequalities in Theorem \ref{thm:norm psd} twice. Suppose the inequalities hold with respect to the OSE $G$ for $AH^THA^T$ and with respect to the OSE $H$ for $AA^T$.
These both happen with probability at least $1-4n\delta$. 
First we have \[\tilde{\ell}(GAH^THA^TG^T)\ge (1-O(\epsilon))\tilde{\ell}(AH^THA^T)
=  (1-O(\epsilon))\tilde{\ell}(HAA^TH^T)\ge (1-O(\epsilon))\tilde{\ell}(AA^T).\] 
Second, 
\begin{align}
(1-O(\epsilon)){\ell}(A)^2 &\le \tilde{\ell}({GAH^THA^TG^T})\nonumber\\
&\le (1+O(\epsilon))\left(\tilde{\ell}(AH^THA^T) + \frac{\tilde{\ell}(I_t)}{t}\sum_{i=d+1}^t\lambda_i(HA^TAH)\right).
\label{eq: qnorm two terms}
\end{align}
The first term on the right hand side of~\eqref{eq: qnorm two terms} can by bounded with Theorem \ref{thm:norm psd} as 
\[
\tilde{\ell}(AH^THA^T) \le (1+O(\epsilon))\tilde{\ell}(AA^T) + (1+O(\epsilon))\left(\frac{\tilde{\ell}(I_d)}{d}\sum_{i=d+1}^n\lambda_i(AA^T)\right).
\]
It remains to bound the second term in \eqref{eq: qnorm two terms}, $\sum_{i=d+1}^t\lambda_i(HA^TAH)$.
We will use a similar proof as used in Lemma 3.5 of \cite{andoni2013eigenvalues},
let $\Lambda_l$ be the $n\times n$ diagonal matrix formed from eigenvalues of $AA^T$ with diagonal entries $(\lambda_1,\ldots,\lambda_d,0,\ldots,0)$ and let
let $\Lambda_s$ be the diagonal matrix with diagonal entries $(0,\ldots,0,\lambda_{d+1},\ldots,\lambda_n)$.
Thus we can write $AA^T = U(\Lambda_l+\Lambda_s)U^T$. Recall that $HU$ is still a $(\epsilon, \delta, d)$-OSE, thus, by Lidskii's Inequality and Lemma \ref{lemma:jlt preserves trace},
\[
\sum_{i=d+1}^t\lambda_i(HA^TAH)\le \tr(HU\Lambda_sU^TH^T)
\le (1+\epsilon)\sum_{i=d+1}^n\sigma_i^2(A).
\]
Thus, with probability at least $1-O(\delta)$,
%By Lemma \ref{fact:gaussian as subspace embedding}, with probability at least $1-1/\poly(n)$, $HA^TG^T$ preserves all the singular values of $A^TG^T$ up to $(1\pm \epsilon)$ factor. 
%Thus with probability at least $1-1/\poly(n)$, $\ell(GAH^THAG^T)=(1\pm \epsilon) \ell(GAA^TG^T)$
%for any fixed unitarily invariant norm $\ell$. Since $\|AA^T\|_{Sp} = \|A\|_{S2p}^2$, by Theorem \ref{thm:norm psd}, we have that with probability at least $1-1/\poly(n)$,
\[
(1-O(\epsilon)){\ell}(A)^2\le \tilde{\ell}({GAH^THA^TG^T})\le (1+O(\epsilon)){\ell}(A)^2 + O\left(\frac{\tilde{\ell}(I_d)}{d}\sum_{i=d+1}^n\sigma_i(A)^2\right).
\]
\end{proof}

\subsection{Lower Bounds}\label{sec: intdim lower bounds}
The complexity
dependence of stable rank or intrinsic dimension (rather than the rank or the actual dimension)
of a matrix
allows us efficient algorithms on matrix norms of matrices that are actually full rank. 
In this section we will show that our algorithm is optimal (up to $\poly(r)$ factor) 
in terms of the intrinsic dimension 
or stable rank of the matrix for all unitarilly invariant norms that satisfy a condition, 
e.g. the Schatten-$p$ norm with  constant $p\notin\{1,2\}$. 
matrix norms.
\begin{theorem}
Fix integer $0\le m\le n$,  $Q$-norm $\ell:\bbR^{n\times n}\rightarrow \bbR$, if for all $t\in[n]$, $t/\ell(I_t)^2\ge t^{\alpha}$ for  some absolute constant $\alpha>0$. Then any $O(1)$-pass streaming algorithm that $(1\pm \epsilon)$-approximates $\ell$ on matrices of stable rank at most $r$ requires 
$\Omega(\poly(r))$ words of space. 
\end{theorem}
\begin{proof}
The proof follows from the vector norm lower bounds. In \cite{braverman2015streaming},
the authors show that the ($O(1)$-pass) streaming space complexity for vector $Q$-norm $\ell$ is $\tilde{\Theta}(t/\ell(I_t)^2)$.  If there is an streaming algorithm for $Q$-norm for matrices, 
we can have an algorithm for the vector $Q$-norm by putting the vector on the diagonal
of a all-zero matrix. For vector of dimension $r$, it is easy to see that the reduction matrix
has dimension at most $r$, and thus of stable rank at most $r$. Therefore, 
the  ($O(1)$-pass)  streaming space complexity of matrix $Q$-norm is 
$\tilde{\Theta}(r/\ell(I_r)^2) = \poly(r)$.
\end{proof}

\begin{theorem}
%{\color{red} To be improved.}
\label{thm:lower bound psd matrix}
Fix integer $0\le m\le n$, constant $0<\alpha <1/2$,  then there exits a unitarilly invariant norm $\ell:\bbR^{n\times n}\rightarrow \bbR$, such that for all $t\in[n]$, $t/\ell(I_t)\ge t^{\alpha}$ and any linear-sketch based streaming algorithm that $(1\pm \epsilon)$-approximates $\ell$ on PSD matrices of intrinsic dimension at most $r$ requires  $\Omega(\poly(r))$ words of space. 
\end{theorem}
This theorem follows from the following lemma since a Schatten-$p$ norm for $1<p<2$ satisfies the conditions of the above lemma. 
\begin{lemma}[A concenquence of \cite{li2014sketching} %{\color{red} Also asked Li Yi for this case, should we cite Yi as personal connection?}
]
Suppose $X\in\bbR^{n\times n}$ is a PSD matrix and $1<p<2$. Suppose that
an algorithm takes $k$ linear sketches of $X$ and computes $Y$ with
$(1-c_p)\|X\|_{S_p}^p\le Y\le (1+c_p)\|X\|_{S_p}^p$ with probability at least $3/4$
then $k=\Omega(\sqrt{n})$, where $c_p$ is a constant depends only on $p$.
\end{lemma}
\begin{proof}
The proof of Theorem 5.4 of \cite{li2014sketching} does not explicitly state
the result for PSD matrices. But we can symmetrize the hard instance matrices as follows.
Suppose the non-symmetric hard instance matrix as $B\in\bbR^{n}$, then define matrix
\[
A=aI_{2n} + \left[
  \begin{array}{cc}
    0 & B^T\\
    B & 0
  \end{array}
  \right],
\]
where $a>1$ is a constant such that with probability at least $0.99$, $A$ is 
a PSD matrix (when $B$ is drawn from the hard distribution).   
The hard distribution is: case 1, $B=(G, GM)$, where $G\in \bbR^{n\times n/2}$
is a column normalized Gaussian matrix, and $M\sim O_{n/2}$; case 2, $B=G'$, 
where $G'\in\bbR^{n\times n}$ is a column normalized Gaussian matrix. For both 
cases, with high probability every non-zero singular values is $\Theta(1)$. Thus it 
is suffice to set $\alpha =\Theta(1)$. Now the norm of $A$ of both distributions 
can be computed exactly using the same formula as (H.15) and (3.4),
and replace their $I_p$ and $J_p$ as follows
i.e. 
\[
I_p'=\int_{0}^4(a+x)^{p/2}\cdot \frac{\sqrt{(4-x)x}}{2\pi x} + \int_{0}^4(a-x)^{p/2}\cdot \frac{\sqrt{(4-x)x}}{2\pi x},
\]
and 
\[
J_p'=2^{p/2}\int_{0}^4(a+x)^{p/2}\cdot \frac{(b-x)(x-a)}{\pi x} +2^{p/2}\int_{0}^4(a-x)^{p/2}\cdot \frac{(b-x)(x-a)}{\pi x}.
\]
Other part of the proof shall follow directly.
\end{proof}

%%% Local Variables: 
%%% mode: latex
%%% TeX-master: "main"
%%% End: 
