# Supplementary material for: Matrix Norms in Data Streams: Faster, Multi-Pass and Row-Order
Source: arXiv:1609.05885 source file (2018-10-24)
Supplement: Supplementary file 2 [file appendix_other.tex]

\section{Unused stuff from the prelims}

%%%%%%%%%%%%%%%%%%%%%%%%% UNUSED STUFF FROM PRELIMS ################################

The above lemma leads to the following useful lemma.
\begin{lemma}
Let $G\in\R^{t\times n}$ be an $(\epsilon, \delta/(2n), 1)$-JLT matrix, 
and let $H\in\R^{t'\times m}$ be an independent $(\epsilon, \delta/(2m), 1)$-JLT 
matrix.
Then the linear map $S: \bbR^{n\times m}\rightarrow \bbR^{t\times t'}$
defined as $S:A\mapsto GAH^T$ is $(6\epsilon, \delta, 1)$-JLT. 
\rnote{The JLT terminology for matrix instead of a vector is confusing. 
I suppose each matrix is viewed flattened into a vector,
and its ``length'' is thus the Frobenious norm 
(and not 2-norm of the matrix, as written in the proof)?
}
\end{lemma}

\begin{proof}
Consider the matrix $A\in \bbR^{n\times m}$ as a vector of dimension $n m$. 
Then 
\[
\|GAH^T\|_2^2=\tr(GAH^THA^TG^T).
\]
Since $AH^THA^T$ is a PSD, by Lemma \ref{lemma:jlt preserves trace}, 
with high probability,
\[
\tr(GAH^THA^TG^T)=(1\pm2\epsilon) \tr(AH^THA^T) = (1\pm 2\epsilon) \tr(HA^TAH^T). 
\]
Applying  Lemma \ref{lemma:jlt preserves trace} again, 
with high probability,
\[
\tr(GAH^THA^TG^T)= (1\pm 2\epsilon) \tr(HA^TAH^T) = (1\pm 6\epsilon)\tr(AA^T). 
\]
Recalling that $\tr(AA^T) = \|A\|_2^2$, the lemma follows by a union bound. 
\end{proof}

\begin{proposition}\label{prop: dot products}
If $S\in\R^{k\times n}$ is an $(\epsilon,\delta,d^2)$-JLT.
Then for every $V\subseteq\R^n$ of cardinality $|V|\leq d$, 
with probability at least $1-\delta$, 
\[
  \forall x,y\in V, \qquad
  - \epsilon\|x\|_2\|y\|_2 
  \leq \tuple{Sx,Sy} - \tuple{x,y}
  \leq \epsilon \|x\|_2\|y\|_2.
\]
\end{proposition}
\begin{proof}
Let $x,y\in V$. 
If $x=0$ or $y=0$ then $\langle x,y\rangle=0=\langle Sx,Sy\rangle$,
hence without loss of generality $\|x\|=\|y\|=1$.
Using the identity 
$\|u+v\|_2^2 -\|u-v\|_2^2 = 4\langle u,v\rangle$, 
we get that 
\[
  4\langle Sx,Sy\rangle-4\langle x,y\rangle =  \|S(x+y)\|_2^2 - \|x+y\|_2^2 + \|x-y\|_2^2 - \|S(x-y)\|_2^2.
\]
Since $S$ is a JLT, the absolute value of the righthand side above is at most 
$ \epsilon(\|x+y\|_2^2+\|x-y\|^2_2) $,
which by the Parallelogram Law (or expanding as inner products), 
is equal to
$ \eps \left( 2\|x\|_2^2 + 2\|y\|_2^2 \right)
  = 4\epsilon$.
\end{proof}
