# Supplementary material for: Matrix Norms in Data Streams: Faster, Multi-Pass and Row-Order
Source: arXiv:1609.05885 source file (2018-10-24)
Supplement: Supplementary file 3 [file appendix_top_eigen.tex]

\section{Proofs from Section \ref{sec:top single values} (Top Singular Values)}
\begin{lemma}
\label{lemma:top eigenvalues}
For $n\ge 1$, let $A\in\bbR^{n\times n}$ be a symmetric matrix and $\lambda^*_i(A)$ be the $i$-th largest 
eigenvalue of $A$ in absolute value. Fix $\epsilon, \phi\in (0,1)$. Let  
$G\in \bbR^{t\times n}$ be both $(O(\epsilon), 1/\poly n, \phi^{-1})$-OSE
and $(0.1, 1/\poly n, \phi^{-1}\eps^{-2})$-OSE.
Then with probability at least $9/10$, the $(\phi^{-1})$-largest eigenvalues of $GAG^T$ in absolute value are $1\pm \epsilon$ multiplicative and $O(\epsilon^2\phi \sum_{i=1/\phi+1}^{n} |\lambda_i^*(A)|  + |\lambda_{1/\phi}^*|)$
additive error approximations of the $\phi^{-1}$ largest eigenvalues of $A$ in absolute value
(under some mapping between the two sets of eigenvalues).
\end{lemma}
Since the proof is similar, we only  point out the necessary changes 
to the proof of \cite[Lemma 3.4]{andoni2013eigenvalues}.
For the full proof, please refer to  proof of \cite[Lemma 3.4]{andoni2013eigenvalues}.
\begin{proof}
By the Spectral Theorem, we can write $A=U^T\Lambda U$, 
where $U$ is an orthormal matrix,
and $\Lambda=\diag(\lambda_1^*, \ldots, \lambda_n^*)$ 
such that $|\lambda_1^*|\ge |\lambda_2^*|\ge \ldots |\lambda_n^*|$.
By Lemma \ref{lemma:ortho trans ose}, also $GU$ is an $(O(\epsilon), 1/\poly n, \phi^{-1})$-OSE matrix
(with the same parameters), 
and thus it suffices to consider a diagonal matrix $A=\Lambda$.  
Now let $\Lambda_i$ ($i\ge 1$) be the diagonal
matrices with eigenvalues of absolute value in the range 
$[|\lambda^*_{1/\phi}(A)|2^{-i}, |\lambda^*_{1/\phi}(A)|2^{-i+1})$
and $\Lambda_0$ be the diagonal matrix of the first $1/\phi$
eigenvalues.
Denote $\Lambda = \sum_{i=0}^{\infty}\Lambda_i$.
By Lemma \ref{lemma:ose preserves eigenvalues},
the non-zero eigenvalues of $G^T\Lambda_0 G$ are $(1\pm \epsilon)$ approximation 
to those of $\Lambda_0$. 
For the rest of the proof to work, we only need to show the additive error term 
$\sum_{i\ge 1}\|G\Lambda_iG^T\|_2$ is small. And it is suffice to show 
that, with probability at least $1-1/\poly(n)$,
for all diagonal matrix $D$ with diagonal entries from $\{0,1\}$,
$\|GDG^T\|_2 \le O(\max(\epsilon^2\phi\tr(D), 1))$.
%\rnote{I could not follow this argument, so it probably should be expanded.
%(1) I suppose the norm on LHS is $S_\infty$, i.e., spectral norm $\norm{.}_2$?
%(2) Do you bound $\ceil{n/d} \le 1+n/d$? 
%(3) You don't say how to use the two OSE assumptions, 
%which indicates you're doing several steps at once...
%}
%\lynote{fixed}
We use the fact that $GU$ is a $(0.1, 1/\poly n, \phi^{-1}\eps^{-2})$-OSE.
By Lemma \ref{lemma:upper bound norm for all norm} we have that,
with probability at least $1-1/\poly n$,
\[
\|GDG^T\|_2\le O(\lceil \epsilon^2\phi\tr(D)\rceil) = O(\max(\eps^2\phi\tr(D), 1)).
\]
%For part 1, by Lemma \ref{lemma:jlt preserves trace} with probability at least $1-1/\poly n$, 
%$\|GDG^T\|_\infty\le 2\tr(D)\le 2n$. For part 2, 
\end{proof}

\begin{lemma}
\label{lemma:singular value heavy hitters}
For $n,m\ge 1$, let $A\in\bbR^{n\times m}$ be an real matrix and $s_i(A)$ be the $i$-th largest 
singular value of $A$. Fix $\epsilon, \phi\in (0,1)$. Let  
$G\in \bbR^{t\times n}, H\in \bbR^{t\times m}$ be independent OSE matrices that
are both of $(O(\epsilon), 1/\poly n, (\phi^{-1}+1))$-OSE and of $(0.1, 1/\poly n, (\phi^{-1}+1)\eps^{-2})$-OSE.
Then with probability at least $9/10$, the $\phi^{-1}$-largest sigular values of $GAH^T$ are $1\pm O(\epsilon)$ multiplicative and $O(\epsilon^2\phi \sum_{i=1/\phi+1}^{n} s_i^2(A)  + s^2_{1/\phi})$
additive error approximations of the $\phi^{-1}$ largest singular values of $A$.
\end{lemma}
We point out  the necessary changes 
to the proof of \cite[Lemma 3.5]{andoni2013eigenvalues}. 
For the full proof, please refer to \cite[Lemma 3.5]{andoni2013eigenvalues}.
\begin{proof}
First note that $A=U\Lambda V^T$, where $\Lambda=\diag(s_1, s_2, \ldots, s_n)$
be the diagonal matrix of singular values. Note that $s_1\ge s_2\ge \ldots s_n\ge 0$.
Now we write $\Lambda=\Lambda_l + \Lambda_s$, where $\Lambda_l$ contains the
top $\phi^{-1}$ singular values and $\Lambda_s$ contains the rest. 
By Lemma \ref{lemma:top eigenvalues}, we have that $\phi^{-1}$ eigenvalues of 
$GAH^THA^TG^T$ are $(1\pm \epsilon)$ approximations to those of $AH^THA^T$
and up to additive error $O(\epsilon^2\phi\sum_{i=\phi^{-1}+1}^n \lambda_i(AH^THA^T) + \lambda_{\phi^{-1}}(AH^THA^T))$. Since $AH^THA^T$ has the same set of eigenvalues
of $HAA^TH^T$. Thus the top $\phi^{-1}$ eigenvalues of $AH^THA^T$ are $(1\pm \epsilon)$ multiplicative approximation to those of $A^TA$ up to $O(\epsilon^2\phi\sum_{i=\phi^{-1}+1}^n \lambda_i(A^TA) + \lambda_{\phi^{-1}}(A^TA))$ additive error. Therefore, it remains to 
show that $O(\epsilon^2\phi\sum_{i=\phi^{-1}+1}^n \lambda_i(AH^THA^T) + \lambda_{\phi^{-1}}(AH^THA^T))$ is upper bounded 
by $O(\epsilon^2\phi\sum_{i=\phi^{-1}+1}^n \lambda_i(A^TA) + \lambda_{\phi^{-1}}(A^TA))$.
First note that, by Lemma~\ref{lemma:top eigenvalues}, with probability at least $1-1/\poly n$,
$\lambda_{\phi^{-1}}(AH^THA^T)) = O(\epsilon^2\phi\sum_{i=\phi^{-1}+1}^n \lambda_i(A^TA) + \lambda_{\phi^{-1}}(A^TA))$.  
By Lidskii inequality and Lemma \ref{lemma:jlt preserves trace}, with probability at least $1-1/\poly n$,
\begin{align}
\sum_{i=\phi^{-1}+1}^n \lambda_i(AH^THA^T) 
&=\sum_{i=\phi^{-1}+1}^n \lambda_i(HA^TAH^T) \nonumber\\
&=\sum_{i=\phi^{-1}+1}^n \lambda_i(HV(\Lambda_l^2 + \Lambda_s^2)V^TH^T) \nonumber\\
&\le \tr(HV\Lambda_s^2V^TH^T)\nonumber \\
&\le (1+O(\epsilon))\tr(\Lambda_s^2).
\end{align}
\end{proof}

%%% Local Variables: 
%%% mode: latex
%%% TeX-master: "main"
%%% End: 
